# Supplementary material for: Few-Shot Learning via Learning the Representation, Provably
Source: arXiv:2002.09434 source file (2021-03-30)
Supplement: Supplementary file 1 [file appendix.tex]

\section{Omitted Proof}

\subsection{Omitted Proof in Kernel Method}

\begin{lemma}
	\label{lemma:move_X}
	For general matrices $X$ and scalar $\lambda$, we have:
	\begin{equation}
	(X^\top X + \lambda I)^{-1}X^\top = X^\top (XX^\top + \lambda I)^{-1}
	\end{equation}
\end{lemma}
\begin{proof}
	Polynomials of the same matrix $X$ commute with each other. In this case, specifically, write SVD of $X$ as $X=U\Sigma V^\top$.
	\begin{align*}
	&(X^\top X + \lambda I)^{-1}X^\top\\
	=& (V(\Sigma^2 + \lambda I)V^\top)^{-1}V\Sigma U^\top \\
	= &V(\Sigma^2 + \lambda I)^{-1}\Sigma U^\top\\
	= & X^\top U\Sigma^{-1}(\Sigma^2 + \lambda I)^{-1}\Sigma U^\top \\
	= & X^\top (XX^\top + \lambda I)^{-1}.
	\end{align*} 	
\end{proof}

\subsection{Kernel Learning with Fixed Design}
For kernel learning, we consider the case when source and target tasks share the same training features $X\in \R^{n\times m}$. We write normalized kernel matrix $K = XX^\top/n$.  

We still have the bias-variance tradeoff on training the source tasks: 
\begin{lemma}
	\label{lemma:kernel_fix}
	For any $\lambda \geq \frac{2}{n_1}\|X^\top Z\|_2 $, where $\lambda$ is the parameter we used to get representation matrix $B$, we have
	\begin{equation*}
	\frac{1}{Tn_1}\|(S_{XB}^{\lambda}-I)X\Theta^*\|_F^2\lesssim\frac{\lambda \|\Theta^*\|_*}{T}, \text{ and }
	\end{equation*}
	\begin{equation*}
	\frac{1}{n}\|S_{XB}^{\lambda}\|_F^2 \lesssim \frac{1}{n}\frac{\|X\|_{2}^2 \|\Theta^*\|_*}{n\lambda}= \frac{\|K\|_2 \|\Theta^*\|_*}{n\lambda}.
	\end{equation*}
\end{lemma} 

For target task we suppose $\theta^*_{T+1}\sim \cD_\theta:=\cN(0,\frac{1}{T}\Theta^*(\Theta^*)^\top)$. 

\begin{theorem}
	\label{thm:kernel_fix}
	For task $T+1$, suppose $\by_{T+1}=X\theta^*_{T+1}+\bz_{T+1}$. 
	We train the model $\bw_{T+1}$ as:
	$$\bw_{T+1}=\min_{\bw}\left\{\frac{1}{2n}\|XB\bw-\by_{T+1}\|_2^2 + \frac{\lambda}{2}\|\bw\|^2\right\}.$$
	%Here $\lambda_c$ makes sure $\|\bw_{T+1}\|\lesssim c:=\sqrt{R/T}$. 
	Then the excess risk is: 
	\begin{align*}
		ER(\bw_{T+1}):=&\E_{\theta_{T+1}\sim \cD_\theta} \frac{1}{n}\|X B\bw_{T+1}-X \theta_{T+1}^*\|^2  \\
		\leq &  \Otil{\|\Theta^*\|_*(\frac{\sqrt{\|K\|_2}}{\sqrt{Tn}}+\frac{\sqrt{\Trace(K)}}{T\sqrt{n}})}.
	\end{align*}
\end{theorem} 
\begin{proof}
Plugging in the solution for $\bw_{T+1}$, we get
	\begin{align*}
		L_{te}(\bw_{T+1}) = & \E_{\theta^*_{T+1}\sim \cD_\theta}\left[\frac{1}{n}\|(S_{XB}^\lambda-I)X\theta^*_{T+1}+S_{XB}^\lambda\bz_{T+1} \|_2^2\right]\\
		\leq &\E_{\theta^*_{T+1}\sim \cD_\theta}\left[ \frac{2}{n}\|(S_{XB}^\lambda-I)X\theta^*_{T+1}\|_2^2+ \frac{2}{n}\|S_{XB}^\lambda\bz_{T+1} \|_2^2 \right]\\
		=& \frac{2}{Tn}\|(S_{XB}^\lambda-I)X\Theta^*\|_F^2+ \frac{2}{n}\|S_{XB}^\lambda\bz_{T+1} \|_2^2
	\end{align*}
For the first term, from Lemma \ref{lemma:kernel_fix}, it is upper bounded by $\frac{\lambda \|\Theta^*\|_*}{T}$. The second term is the $\ell_2$ norm of a vector that follows Gaussian distribution $\cN(0, \frac{1}{n}(S_{XB}^\lambda)^2)$. Therefore with probability $1-\delta$, $\frac{2}{n}\|S_{XB}^\lambda\bz_{T+1} \|_2^2 \leq \Otil{\frac{1}{n}\|S_{XB}^\lambda\|_F^2}\leq \Otil{\frac{\|K\|_2}{n}\frac{\|\Theta^*\|}{n\lambda}}$. 

By Lemma \ref{lemma:bound_lambda} we need to set $\lambda \geq \Otil{\frac{1}{\sqrt{n}}(\sqrt{T}\sqrt{\|K\|_2}+\sqrt{\Trace(K)})}$. Notice that when $\lambda\geq \Otil{\sqrt{\frac{T\|K\|_2}{n}}}$, the first term is dominating. Therefore we get with probability $1-\delta$, $\frac{2}{Tn}\|(S_{XB}^\lambda-I)X\Theta^*\|_F^2+ \frac{2}{n}\|S_{XB}^\lambda \bz_{T+1}\|_2^2 \leq  \Otil{\frac{\lambda\|\Theta^*\|_*}{T}}\leq \Otil{\|\Theta^*\|_*(\frac{\sqrt{\|K\|_2}}{\sqrt{Tn}}+\frac{\sqrt{\Trace(K)}}{T\sqrt{n}})}$.  
\end{proof}
